# Supplementary material for: Smart Contract Development from the Perspective of Developers: Topics and Issues Discussed on Social Media
Source: arXiv:1905.08833 source file (2020-01-17)
Supplement: Supplementary file 1 [file appendix.tex]

\clearpage
\section{Discussion Trends}
\label{app:trends}

%Usually, the Medium posts are similar to the blog posts and readers/followers provide feedback as responses. According to our survey, most of the posts do not contain any response and the rest one-third contains different number of responses. We also look into the reading time of each post to understand the length of the post and to understand how much details are available thereby. 

Figure~\ref{fig:medium_response_read} shows the distributions of the number of responses and of reading time for smart contract related posts on Medium. Please note the logarithmic scale on the vertical axis. %In both cases, we represent the number of posts in logarithmic scale. 

\iffalse
\begin{figure}[ht]
  \subfloat[According to number of responses]{
	\begin{minipage}[c][1\width]{
	   0.55\textwidth}
	   \centering
	   \includegraphics[width=1\textwidth]{images/medium_response_count.pdf}
	\end{minipage}}
 \hfill 	
  \subfloat[According to the Reading time]{
	\begin{minipage}[c][1\width]{
	   0.55\textwidth}
	   \centering
	   \includegraphics[width=1.1\textwidth]{images/medium_read_time.pdf}
	\end{minipage}}
 \hfill	
 \caption{Number of posts based on the response count and Reading time.}
 \end{figure}
\fi

\begin{figure}
    \centering
    \includegraphics[width=\textwidth]{images/medium_response_read.pdf}
    \vspace{-2em}
    \caption{Number of Medium posts based on the response count and Reading time.}
    \label{fig:medium_response_read}
\end{figure}

\clearpage
\section{Discussion Topics}
\label{app:topics}

\begin{figure}
\includegraphics[width=\textwidth]{images/SO_Popular_Tags.pdf}
\caption{Popularity of various tags in smart contract related questions on Stack Exchange, measured as frequency usage and total scores, answers, and comments.} 
\label{fig:SO_Popular_Tags}
\end{figure}

\begin{figure}
    \centering
    \includegraphics[width=\textwidth]{images/medium_tag_interest.pdf}
    \caption{Popularity of various tags in smart contract related posts on Medium, measured as frequency usage and total number of claps, voters, and responses.}
    \label{fig:medium_tag_interest}
\end{figure}

\begin{figure}
\includegraphics[width=\textwidth]{images/SO_Trends_of_Tags.pdf}
\caption{Number of questions posted on Stack Exchange with various tags each month.} \label{fig:SO_Trends_of_Tags}
\end{figure}

\begin{figure}
    \centering
    \includegraphics[width=\textwidth]{images/medium_trends_of_tags.pdf}
    \caption{Number of posts on Medium with various tags each month.}
    \label{fig:medium_tag_trends}
\end{figure}

\clearpage
\section{Developers}
\label{app:developers}

\subsubsection{Location of Users}
On Stack Exchange, users may specify their real-world locations.
Among the 55,351 smart contract developers, 18,422 had specified their location in some form. We used the HERE Maps API\footnote{HERE Maps API: \url{https://developer.here.com/products/maps}} to translate these locations into complete addresses, and then we group the users based on to their countries (Figure~\ref{fig:SO_LocationComparison}). 
We find that the United States and India have the largest number of users, with 4078 and 2543 users, respectively. 
For comparison, we took a random 1\% sample of all Stack Overflow users. We find that the location distribution is very similar to that of smart contract developers, with the United States and India again having the most of users.  

\begin{figure}[h]
\includegraphics[width=\textwidth]{images/SO_LocationComparison.pdf}
\caption{Location of smart contract developers and other Stack Overflow users.} \label{fig:SO_LocationComparison}
\end{figure}

\subsubsection{Statistics of Medium Authors}

\paragraph{Experience and Professionalism}
We find 1562 individual authors on Medium who write on smart contracts or associative tools and topics. Most of the authors from Medium are experienced bloggers who have more than 10 posts. Almost  83\%  authors  have  bio's  and  most  of  which  approximately  45\%  bio's  include  any  of  the  following words- ethereum, smart contracts, solidity, web3, ether etc. The stat is interesting and reveals the professionalism of the authors. It is also noticeable that 62\% of the authors mention their twitter username in their profiles. Figure~\ref{fig:medium_author_post_count} indicates the experience of the authors using their post count in the profile. 
\begin{figure}[h]
    \centering
    \includegraphics[width=0.8\textwidth]{images/medium_author_post_count.pdf}
    \caption{Number of posts for Medium authors}
    \label{fig:medium_author_post_count}
\end{figure}

\paragraph{Reputation of Authors}
Later we figure out the reputation of the authors who use different tags in their writing based on the number of their follower count. Also, their interactivity is represented based on the number of other authors they follow in Medium. Figure~\ref{fig:medium_author_popularity} represents the author profile analysis based on the follower and following count. According to the survey, we find most of the authors to have around 1200 followers on average who write on smart contract related posts. This indicates that the Medium community has approximately the same number of other authors or Medium users who are likely to get updates on smart contract related posts. We also find the difference of interests between two popular smart contract language- Solidity and Vyper. It seems that the authors publish posts on Solidity has a higher reputation than the ones who write on Vyper.

\begin{figure}[h]
    \centering
    \includegraphics[width=\textwidth]{images/medium_author_reputations.pdf}
    \caption{Reputation and interactivity analysis of Medium authors who use different tags}
    \label{fig:medium_author_popularity}
\end{figure}

\clearpage
\section{Common Security Issues and Tools}
\label{app:security}

\begin{figure}[h]
    \centering
    \includegraphics[width=\textwidth]{images/medium_Trend_for_Reentracy_Security_Vulnerability.pdf}
    \caption{Number of smart contract related posts per month on Medium mentioning \emph{reentrancy} and \emph{security} or \emph{vulnerability}.}
    \label{fig:medium_Trend_for_Reentracy_Security_Vulnerability}
\end{figure}

\begin{table}[h]
\caption{Co-Occurrence of Security Issues and Tools}
\centering
\resizebox{\textwidth}{!}{
    \begin{tabular}{|c||c|c|c|c||c|c|c|}
    \hline
   Security Issues &  Security Tools & SO & Medium & Security Issues &  Security Tools & SO & Medium\\
    
    \hline
    \hline
    \multirow{15}{*}{\shortstack{Security /\\Vulnerability}} &  Mythril & 6 & 68 & \multirow{15}{*}{Re-Entrancy} &  Oyente & 2 & 32\\
    \cline{2-4}\cline{6-8}
    & Securify & 4 & 35 & & Mythril & 2 & 29\\
    \cline{2-4}\cline{6-8}
     & Ethlint/Solium & 4 & 22 & &  Manticore & 1 & 4\\
     \cline{2-4}\cline{6-8}
    & Manticore & 3 & 15 & & Securify & 1 & 22\\  
     \cline{2-4}\cline{6-8}
    & Oyente & 6 & 51 & & solcheck & 1 & 1\\  
     \cline{2-4}\cline{6-8}
     & Smartcheck & 3 & 46 & & solgraph & 1 & 3\\  
     \cline{2-4}\cline{6-8}
    & Ethir & 2 & 1 & & solhint & 1 & 25\\  
     \cline{2-4}\cline{6-8}
    & Solcheck & 2 & 4 &  & solint & 1 & 1\\  
     \cline{2-4}\cline{6-8}
    & Solgraph & 2 & 6 & &  Ethlint/Solium & 1 & 8\\  
     \cline{2-4}\cline{6-8}
    & Solint & 2 & 3 & & Sonarsolidity & 1 & 0\\  
     \cline{2-4}\cline{6-8}
    & Solhint & 2 & 29 & & Smartcheck & 0 & 35\\  
     \cline{2-4}\cline{6-8}
    & Sonarsolidity & 2 & 0 & & Scompile & 0 & 27\\  
     \cline{2-4}\cline{6-8}
    & Teether & 2  & 1 & & Slither & 0 & 4\\  
     \cline{2-4}\cline{6-8}
    & Vandal & 2 & 1 & & Surya & 0 & 2\\ 
    \cline{2-4}\cline{6-8}
    & Contractfuzzer & 1 & 1 & & Contractfuzzer & 0 & 1\\ 
    \cline{2-4}\cline{6-8}
    & Scompile & 0 & 27 & & Sasc & 0 & 1\\
    \cline{2-4}\cline{6-8}
    & Surya & 0 & 6 & & Verisolid & 0 & 1\\
    \cline{2-4}\cline{6-8}
    & Slither & 0 & 6 & & Maian & 0 & 2\\
    \cline{2-4}\cline{6-8}
    & Verisolid & 0 & 1 && Ethir & 0 & 1\\
    \cline{2-4}\cline{6-8}
    \hline
    \hline
    
    \multirow{11}{*}{\shortstack{Timestamp\\Dependency}} &  Mythril  & 2 & 16 &
     \multirow{11}{*}{\shortstack{Transaction\\Ordering\\Dependency}} & Mythril & 2 & 16\\
    \cline{2-4}\cline{6-8}
    & Ethlint/Solium & 1 & 3 & & Ethlint/Solium  &  1 & 3\\  
     \cline{2-4}\cline{6-8}
    & Manticore & 1 & 0 & & Manticore  &  1 & 0\\  
     \cline{2-4}\cline{6-8}
    & Oyente & 1 & 2 & & Oyente & 1 & 2\\  
     \cline{2-4}\cline{6-8}
    & Securify & 1 & 1 & & Securify & 1 & 1\\  
     \cline{2-4}\cline{6-8}
    & Smartcheck & 1 & 2 & & Smartcheck & 1 & 1\\  
     \cline{2-4}\cline{6-8}
    & Solcheck & 1 & 0 & & Solcheck & 1 & 0\\  
     \cline{2-4}\cline{6-8}
    & Solgraph & 1 & 0 & & Solgraph & 1 & 0\\  
     \cline{2-4}\cline{6-8}
    & Solint & 1 & 0 & & Solint & 1 & 0\\  
     \cline{2-4}\cline{6-8}
    & Solhint & 1 & 0 &  & Solhint & 1 & 1\\  
     \cline{2-4}\cline{6-8}
    & Sonarsolidity & 1 & 0 & & Sonarsolidity & 1 & 0\\ 
    \cline{2-4}\cline{6-8}
    & Maian & 0 & 1 && Sasc & 0 &1 \\
    \cline{2-4}\cline{6-8}
    & Sasc & 0 & 1 && Slither & 0 & 1\\
    \cline{2-4}\cline{6-8}
    & Slither & 0 & 1 && Maian & 0 & 1\\
    \hline
    
    \end{tabular}}
\label{tab:Co_Occurance}
\end{table}
